# Supplementary material for: X-3D: Explicit 3D Structure Modeling for Point Cloud Recognition
Source: arXiv:2404.15010 source file (2024-04-23)
Supplement: Supplementary file 1 [file X_suppl.tex]

\clearpage
\setcounter{page}{1}
\maketitlesupplementary
\section{Supplementary Material on Sec~\ref{sec: manifold}}
\subsection{Manifold Learning}
There are two views of manifold learning, ISOMAP optimizes by minimizing the distance vector between the embedding space and the input space, and its procedure can be written as:
\begin{equation}
\label{eq:isomap}
    \mathop{argmin}\limits_{B}\sum_{i,j}||dist_A(A_i,A_j),dist_B(B_i,B_j)||
\end{equation}
where $dist_A$  usually stands for a distance metric such as geodesic distance that conforms to the properties of the underlying manifold in original space A, while $dist_B$ usually refers to Euclidean distance in the embedding space B.

Then, LLE works by minimizing the local structure of the embedding space and the input space:
\begin{equation}
    \label{eq:lle}
    ES=\mathop{argmin}\limits_{ES}\sum_{i=1}^N||A_i-\sum_{j=1}^kES_{i,j}A_{i,j}||
\end{equation}

Then the embedding space B is obtained by satisfying the linear reconstruction relation, which means that the LLE generates a mapping from original input to embedding through the geometric local structure:
\begin{equation}
    B=\mathop{argmin}\limits_{B}\sum_{i=1}^N||B_i-\sum_{j=1}^KES_{i,j}B_{i,j}||
\end{equation}

By the comparison of Eq \ref{eq:isomap} and Eq \ref{eq:ls_vector}, Eq~\ref{eq:lle} and Eq~\ref{eq:ls_structure}, it can be seen that whether explicit local structure is used in the process of embedding relation vectors is the main difference between the two methods, so LLE provides some interpretability for the efficient performance of X-3D.

\subsection{Manifold in Point Clouds.}
Point cloud is a typical manifold data, so many works~\cite{gppcs,lang2021deepume,pointmanifoldcut,yang2020pointmanifold,pdmm,approximating}directly apply manifold learning to point cloud tasks.  GP-PCS~\cite{gppcs} employs Gaussian processes suitable for functions defined on Riemannian manifolds to model the surface on the point cloud. DeepUME~\cite{lang2021deepume} directly uses manifold embedding to complete point cloud registration. PointManifold~\cite{yang2020pointmanifold} decomposes the 3D point cloud neighborhood into three 2D manifolds and extracts features separately. ~\cite{pdmm,approximating} believe that it is more important to use distance embeddings in manifold space such as geodesic distance instead of Euclidean embeddings.

Inspired by these works, we argue that existing works  may learn a mapping from Euclidean embeddings to manifold embeddings by stacking a large number of MLPS,  which is similar to manifold learning. In Fig~\ref{fig:challenge}, we compare the similarity between geometric correlations captured by existing ISHM models and geodesic distances, which further proves the association of IHSM with ISOMAP.

\begin{figure}[!h]
\vspace{-1.1em}
\includegraphics[width=1\linewidth]{image/sim_geo_pe.pdf}
\vspace{-1em}
\caption{We compare the similarity between geometric correlations captured by existing ISHM models and geodesic distances, and can find that existing works implicitly learn a mapping from Euclidean embeddings to manifold embeddings and capture local structure through manifold embeddings. ).
}\label{fig:challenge}
\end{figure}

However, from the Fig~\ref{fig:challenge}, we can see that even though the learning difficulty can be reduced by adding additional surface information, such as RepSurf curvature, etc., as analyzed in sec~\ref{sec: manifold} , due to the lack of explicit local structure, it is still very difficult to directly learn the Euclidean embedding to the manifold embedding (the similarity is only  about 84\%).

\section{Examples of Implict High-dimensional Structure Modeling}
In this section, we will detail some representative works on implict high-dimensional structure modeling. There are mainly two key parts, one is how to construct the relation vector, and the other is to generate the dynamic embedding kernel for the relation vector.

\textbf{PointNet++}~\cite{pointnet++} and \textbf{PointMetaBase}~\cite{lin2023meta} simply treat the relative coordinate difference as a relation vector:
\begin{equation}
   V_{i,j}=\mathbf{p}_i-\mathbf{p}_{i,j}
\end{equation}

\textbf{RandLA}~\cite{hu2020randla} additionally introduces absolute coordinates and Euclidean distances:
\begin{equation}
   V_{i,j}=(\mathbf{p}_i-\mathbf{p}_{i,j}, \mathbf{p}_i, \mathbf{p}_{i,j}, ||\mathbf{p}_i-\mathbf{p}_{i,j}||^2_2)
\end{equation}

\textbf{GAM}~\cite{hu2023gam} proposes a simplified depth gradient information as the relation vector:
\begin{equation}
   \mathbf{p}_i-\mathbf{p}_{i,j}=(\mathop{x_{i,j}}\limits ^{\rightarrow},\mathop{y_{i,j}}\limits ^{\rightarrow},\mathop{z_{i,j}}\limits ^{\rightarrow})
\end{equation}
\begin{equation}
   V_{i,j}=(\frac{\mathop{z_{i,j}}\limits ^{\rightarrow}}{||\mathbf{p}_i-\mathbf{p}_{i,j}||^2_2}\frac{\mathop{x_{i,j}}\limits ^{\rightarrow}+\mathop{y_{i,j}}\limits ^{\rightarrow}}{\sqrt{(\mathop{x_{i,j}}\limits ^{\rightarrow})^2+(\mathop{y_{i,j}}\limits ^{\rightarrow})^2}}, ||\mathbf{p}_i-\mathbf{p}_{i,j}||^2_2)
\end{equation}

\textbf{RepSurf}~\cite{repsurf} is special. Although it captures surface information at the beginning, as the down-sampling rate becomes larger, the point cloud becomes sparse, and the initial surface information can only describe points, but cannot characterize the neighborhood structure.
\begin{equation}
   V_{i,j}=[\mathbf{p}_i-\mathbf{p}_{i,j},n_{j},n_{j}^T\mathbf{p}_{i,j},S_{i,j}]
\end{equation}
where $n_{j}$ represents the normal vector of the $j$-th point and $S_{i,j}$  means the coordinate of the $j$-th point in the spherical coordinate system with point $i$ as the center.

Then for vector kernel, most methods like PointNet++~\cite{pointnet++}, PointNeXt~\cite{pointnetxt} and so on directly use shared-weight MLP to implicitly embed the relation vector:
\begin{equation}
    \mathcal{M}(\mathbf{W}_{i,j},\mathbf{f}_{i,j},V_{i,j})=MLP(V_{i,j},f_{i,j})
\end{equation}
At the same time, there are also many methods such as PointMetaBase~\cite{lin2023meta}, RepSurf~\cite{repsurf}, etc. that explicitly use shared-weight MLP to embed relationship vectors:
\begin{equation}
    \mathcal{M}(\mathbf{W}_{i,j},\mathbf{f}_{i,j},V_{i,j})=MLP(V_{i,j})+MLP(f_{i,j})
\end{equation}

\textbf{RSConv}~\cite{relation-shape} uses MLP to generate dynamic kernels based on relation vectors:
\begin{equation}
   \mathbf{W}_{i,j}=MLP(V_{i,j})
\end{equation}
\begin{equation}
    \mathcal{M}(\mathbf{W}_{i,j},\mathbf{f}_{i,j},V_{i,j})=MLP(\mathbf{W}_{i,j}*\mathbf{f}_{i,j})
\end{equation}

\textbf{KPConv}~\cite{kpconv} dynamically generates kernels based on geometric relationships between neighborhood points and predefined kenrel points:
\begin{equation}
   \mathbf{W}_{i,j}=\sum_{k=1}^rh(\mathbf{p}_{i,j},\mathbf{\widetilde{p}}_k)\mathbf{G}_k
\end{equation}
\begin{equation}
   \mathcal{M}(\mathbf{W}_{i,j},\mathbf{f}_{i,j},V_{i,j})=\mathbf{W}_{i,j}\mathbf{f}_{i,j}
\end{equation}
where $\mathbf{\widetilde{p}}_k$ and $\mathbf{G}_k$ represent the coordinates and weights of the $k$-th predefined kernel points, and $r$ means the number of kernel points. $h$ represents the geometric distance between kernel point and neighborhood point.

It can be seen that these methods implicitly capture the local structure in the high-dimensional space through the relation vector, so they pay more attention to how to construct a good relation vector $V_{i,j}$ and how to generate a good vector kernel $\mathbf{W}_{i,j}$ for the relation vector

\begin{algorithm}[t]
\caption{Pytorch-Style Pseudocode of PointHop}
\label{alg:pointhop}
\definecolor{codeblue}{rgb}{0.25,0.5,0.7}
\vspace{-4pt}
\lstset{
  backgroundcolor=\color{white},
  basicstyle=\fontsize{7.6pt}{7.6pt}\ttfamily\selectfont,
  columns=fullflexible,
  breaklines=true,
  captionpos=b,
  commentstyle=\fontsize{10pt}{10pt}\color{codeblue},
  keywordstyle=\fontsize{10pt}{10pt},
}
\begin{lstlisting}[language=python]
# b: batch size, n: number of center points
#k: number of neighbor points, c: feature channels
#p:  coordinates of input point cloud  (b,n,k,c)
partion_idx=(p[...,0]>0)*4+(p[...,1]>0)*2+(p[...,2]>0)
centroid=scatter_mean(p,idx=partion_idx)
centroid=concat(centroid,dim=-1)
return centroid
\end{lstlisting}
\vspace{-3pt}
\end{algorithm}

\begin{algorithm}[!t]
\caption{Pytorch-Style Pseudocode of Neighborhood Context Propogation}
\label{alg:ncp}
\definecolor{codeblue}{rgb}{0.25,0.5,0.7}
\vspace{-4pt}
\lstset{
  backgroundcolor=\color{white},
  basicstyle=\fontsize{7.6pt}{7.6pt}\ttfamily\selectfont,
  columns=fullflexible,
  breaklines=true,
  captionpos=b,
  commentstyle=\fontsize{10pt}{10pt}\color{codeblue},
  keywordstyle=\fontsize{10pt}{10pt},
}
\begin{lstlisting}[language=python]
# b: batch size, n: number of center points
#k: number of neighbor points, c: feature channels
#f:  input point cloud
#fps_idx: index of the center points
group_idx=ball query(f) #b,n,k
f=grouping&modeling(f,group_idx)  #b,n,k,c
f_0=Maxpooling(f) #b,n,c

f_1=scatter_mean(f.view(b,-1,c),dim=1,index=group_idx.view(b,-1))
f_1=gather(f_1,fps_idx)

f_2=MLP([f_0,f_1])
return f_2
\end{lstlisting}
\vspace{-3pt}
\end{algorithm}

\section{Implementation of X-3D}
In this part, we detail a part of the implementation of X-3D. 

% First, since X-3D can be embedded into existing models, it is necessary to explore at which layers X-3D is applied. We analyze the characteristics of the shallow and deep layers of the model. As shown in Table~\ref{tab:diff_supp}, we find that as the  network layers becomes deeper and deeper, the difference between the implicit local structure of feature space and the explicit local structure of 3D space becomes larger and larger, which means that the geometric information is lost more and more seriously, \textbf{so the deep layer needs the explicit 3D local structure brought by X-3D}.

% \begin{table}[!h]

% \centering
% \caption{ We tested the difference between the implicit local structure of the feature Spaces at different layers and the explicit space of the input 3D space}
% % We report the average$\pm$std in three random runs.
% \label{tab:diff_supp}

% \resizebox{0.9\linewidth}{!}{
%  \setlength{\tabcolsep}{2.5pt}
% \begin{tabular}{c|cccc}

% &layer1&layer2&layer3&layer4\\
% \midrule
% GAP&2.16&4.23&5.37&7.02\\
% \bottomrule
% \end{tabular}
% }
% % \caption{\textbf{Ablation Study of PointMLP(ours) on different training strategies.}
% \end{table}

First, we introduce the implementation algorithm of PointHop which is shown in Algorithm~\ref{alg:pointhop}, we use the scatter operator to  compute the centroid of each partition.

Then, We detail the specific implementation of neighborhood context propagation which is shown in Algorithm~\ref{alg:ncp}. We use the scatter operator to fuse the features of each point in different neighborhoods (either as a center point or as a neighboring point), and then select only the center point's fused feature as the propagated feature. 

\section{Additional Analysis of NCP}
In this part, we conduct detailed analysis and ablation experiments for Neighborhood Context Propagation.

Firstly, from the perspective of computation, NCP simply uses the overlapping region to propagate context information and expand the receptive field, which saves a lot of computation compared with simply expanding the neighborhood range~\cite{lai2022stratified}. 

Then we  compared methods for different propagation contexts which is shown in Fig~\ref{fig:diff_ncp}. After calculating the features of each point through the attention mechanism, LCPFormer first propagates the context information through context agg, and then performs local agg to aggregate the features in the neighborhood. RandLA first performs local agg to extract local features after obtaining the neighborhood by grouping, and then performs another grouping to carry out context agg to propagate context information with the local features obtained in the previous step. In X-3D, we believe that local agg captures fine local details, while context agg captures coarse global information. In order to balance the role of the two steps, we discard the sequential execution of the two steps, but perform them in parallel, and fuse the two information through an adaptive aggregation module.

\begin{figure}[!h]
 \begin{subfigure}[t]{0.45\linewidth}
           \centering
           \includegraphics[width=\textwidth]{image/randla.pdf}
            \caption{RandLA}
           
\end{subfigure}
\begin{subfigure}[t]{0.45\linewidth}
           \centering
           \includegraphics[width=\textwidth]{image/expand.pdf}
            \caption{Expand}
            
\end{subfigure}
\begin{subfigure}[t]{0.45\linewidth}
           \centering
           \includegraphics[width=\textwidth]{image/lcpformer.pdf}
            \caption{LCPFormer}
            
\end{subfigure}
\begin{subfigure}[t]{0.5\linewidth}
        \centering
        \includegraphics[width=\textwidth]{image/X-3D.pdf}
       \caption{X-3D}
        
\end{subfigure}

\caption{We visualize how different methods propagate the neighborhood context. We can see that previous methods usually execute context agg and local agg in a different order or directly expand the neighborhood to execute both. X-3D executes the two steps in parallel, which not only preserves the fine local details of the current region but also fuses the context information
}\label{fig:diff_ncp}
\vspace{-1.1em}
\end{figure}

Furthermore, we can see that we only propagate the context information including the center point, which effectively limits the scope of propagation and avoids conflicts caused by large differences between local structures in different regions.

Finally, to demonstrate the effectiveness of the above design, we conduct ablation experiments of NCP on S3DIS Area5. We can see that the parallel local agg and context agg provide the model with the structure to deal with context flexibly. At the same time, by limiting the propagation range, the conflict between local structures is avoided, which effectively improves the performance of NCP

\begin{table}[!h]

\centering
\caption{We tested NCP on S3DIS, where L$\rightarrow$C stands for local agg followed by context agg, L\& C stands for performing both steps in parallel, and Includ-Center stands for propagating only context information containing the center point}
% We report the average$\pm$std in three random runs.
\label{tab:ncp_ablation}

\resizebox{\linewidth}{!}{
 \setlength{\tabcolsep}{2.5pt}
\begin{tabular}{cccc|c}
\toprule
L$\rightarrow$ C&C$\rightarrow$ L&L\& C&Include-Center&mIoU\\
\midrule
&&\checkmark&\checkmark&\textbf{71.9}\\
\checkmark&&&\checkmark&71.2\\
&\checkmark&&\checkmark&70.9\\
&&\checkmark&&71.6\\
\bottomrule
\end{tabular}
}
\end{table}

\section{Additional Analysis of ES }
In this section, we first introduce several explicit local structures in depth and detail their properties. Then we analyze the reasons for the excellent performance of X-3D in detail for the viewpoints of ES properties.
\subsection{Properties}

First we present the implementation of different explicit local structures:

\textbf{LR.} LLE~\cite{roweis2000nonlinear}  proposes local linear relations (LR) as explicit local structures which is shown in Eq~\ref{eq:lle},
 % From the Eq~\ref{eq:lle}, we can see that the composition of $ES$ is affected by the order of the points, so it lacks the property of \textbf{Symmetry}. At the same time, because the linear relationship well describes the information in the local neighborhood, LR has a stronger \textbf{Internal Detail} property.

\textbf{PCA.} \cite{pca,spg} proposed to obtain an explicit local structural descriptor by performing pca on the local neighborhood and combining the eigenvalues and eigenvectors. Specifically, for eigenvectors ($e_1$,$e_2$,$e_3$) and eigenvalues ($\lambda_1$,$\lambda_2$,$\lambda_3$), we can describe the overall shape by linear, planar, and scatter:
\begin{equation}
    linear=\frac{\lambda_1-\lambda_2}{\lambda_1}, \quad  planar=\frac{\lambda_2-\lambda_3}{\lambda_1}, \quad scatter=\frac{\lambda_3}{\lambda_1}
\end{equation}

\textbf{PH.} PointHop~\cite{zhang2020pointhop} partitions the point cloud neighborhood into fixed octets and computes the centroid of each partition. The process of PH we have described in detail in Eq~\ref{eq:pointhop}.
% In addition, the information of perpendicularity and entropy with the horizontal line is also taken into account. It can be seen that the PCA method mainly highlights the shape and motion direction of the overall local area, so it is more prominent in the \textbf{Overall Shape} attribute.

Then, we then detail the different properties:

\textbf{Symmetry.} Since the point cloud is unordered, an effective $ES$ should possess symmetry and not be affected by the order of the point cloud.
According to the above formula, we can see that the linear relation $ES$ defined by LLE is obviously affected by the order of the points, so its property of symmetry is missing.

\textbf{Gloabl Shape.} The global shape of a local region describes the overall shape information, such as sphere, cuboid, etc., which provides a good geometric prior for the region category. Traditional point cloud analysis methods can usually identify the object shape information by the main direction of the data. For example, PCA provides explicit information about the principal directions directly, whereas PointHop, like ~\cite{hastie1989principal}, provides the overall principal directions by partitioning the regions and computing the centroids of the regions. However, although LLE explicitly provides the orientation of all neighborhood points, it is difficult to directly extract the overall main orientation, so the property of global shape is missing.

\textbf{Local Detail.} The global shape above provides a simple geometric prior, but the detailed information inside the local region is missing, so we believe that a valid $ES$ should also have the property of A. PCA uses three eigenvalues and eigenvectors to describe the overall shape, but it lacks information about the internal neighborhood points, so the local detail property is missing.

 We believe that LR pays more attention to the local information of each point detail in the local structure, PCA pays more attention to the global information in the local structure, and PH is a better balance between the internal details and the overall shape.

\subsection{Reasons}
\textbf{Global Shape provides a good geometric prior for category learning in local regions.} This part has been described in detail in the main text.

% \begin{figure}[!t]
%     \centering
%     \begin{subfigure}[t]{0.15\textwidth}
%            \centering
%            \includegraphics[width=\textwidth]{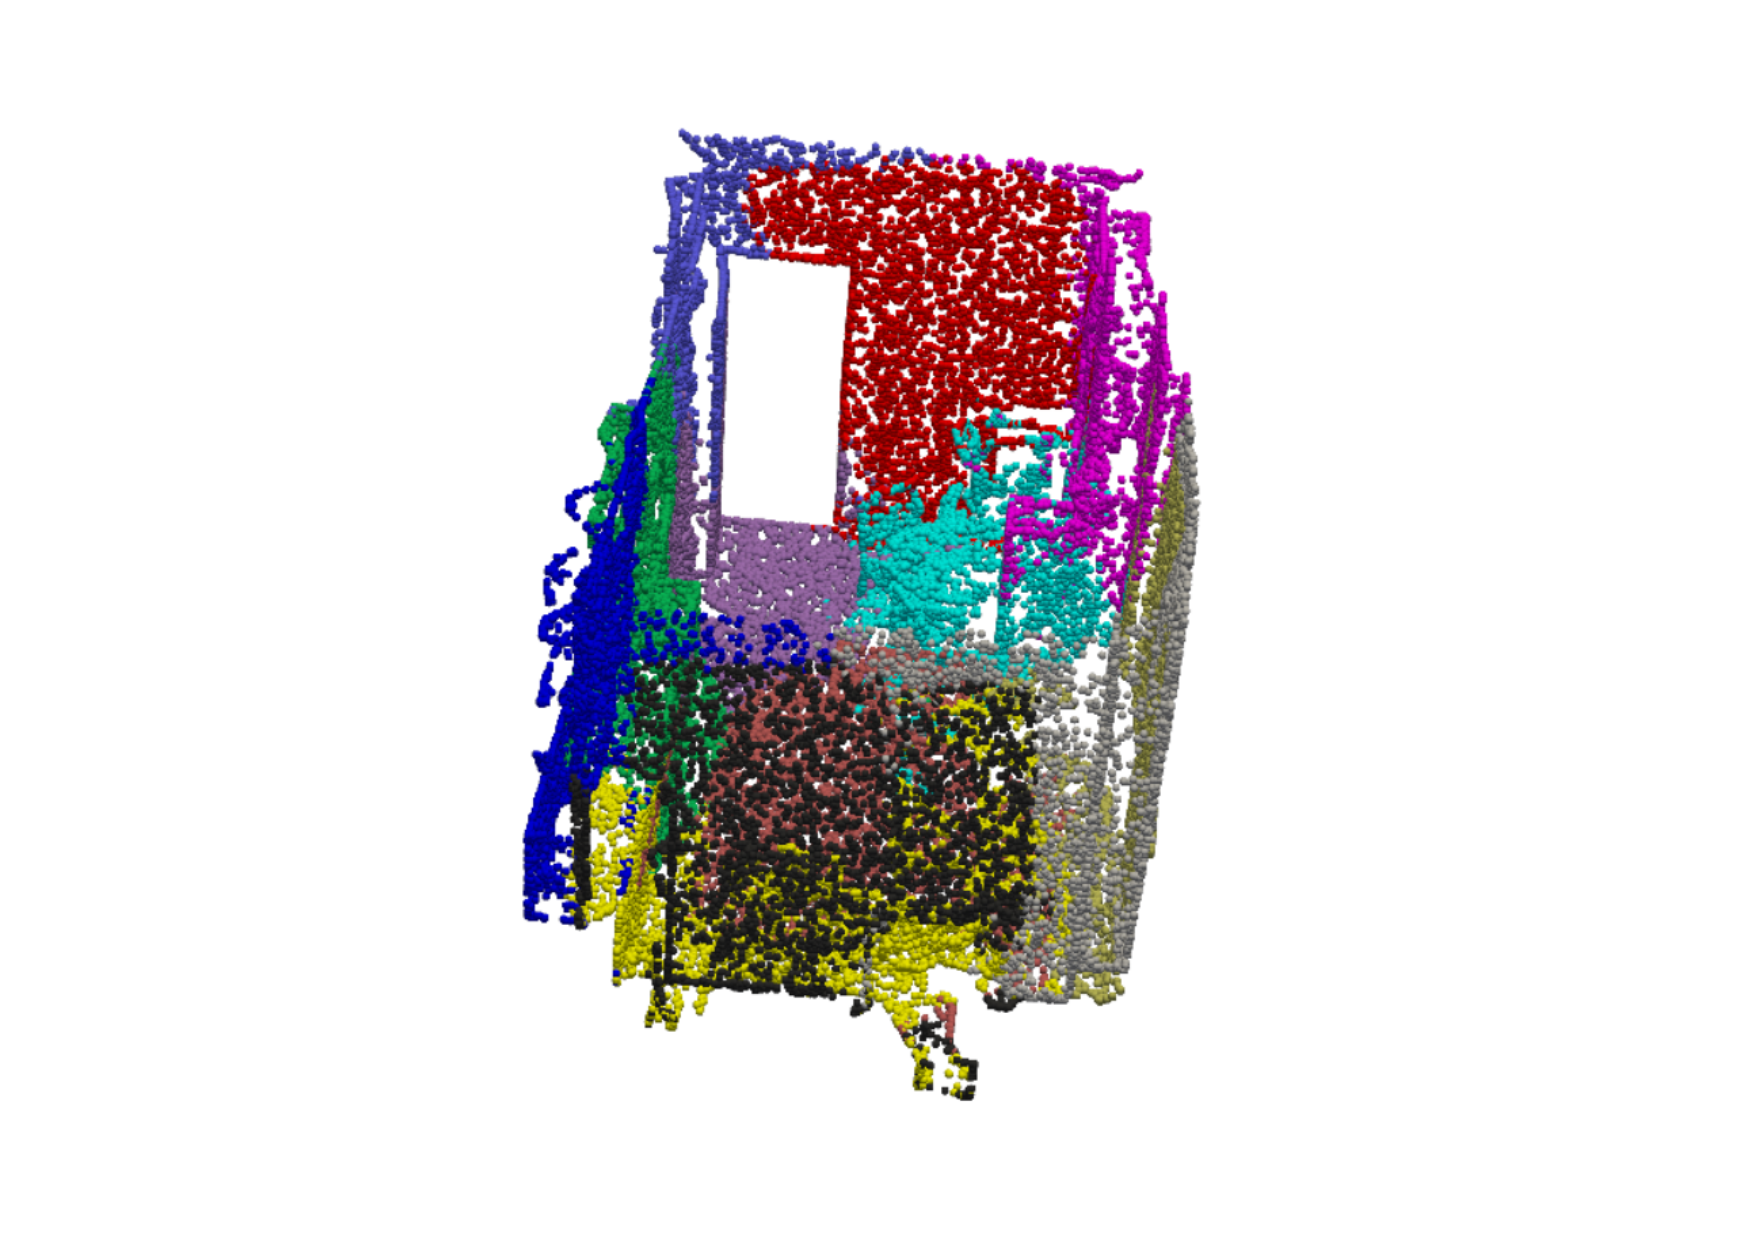}
%            \caption{}
           
%     \end{subfigure}
%     \begin{subfigure}[t]{0.15\textwidth}
%             \centering
%             \includegraphics[width=\textwidth]{image/vis_scene2.pdf}
%             \caption{}

%     \end{subfigure}
  
%     \caption{Visualization of the Structure Kernel}
%     \label{fig:vis}
%     \vspace{-1.1em}
% \end{figure}

\textbf{Local Details provide richer geometric informations.} To demonstrate that local details provide richer geometric information for each neighborhood point, we design tasks to predict geodesic distance, normal vector, relative position which is shown in Table~\ref{tab:geo_predict} , and the performance of these tasks demonstrates the richness of geometric information

We predict those geometric metric of neighborhood points based on the aggregated local structures and neighborhood point features which can be written as follow:
\begin{equation}
   Predict=MLP([\hat{\mathbf{f}}^{(2)}_i,\mathbf{f}_{i,j}])
\end{equation}

For relative coordinates, direct prediction is difficult, inspired by PointRCNN~\cite{pointrcnn}, we adopt a bin-based strategy, that is, the relative coordinates are divided into bins according to the maximum and minimum values, and predict which bin it is in, which turns into a classification task, and we report the classification accuracy of this task.

Then for normal vectors and geodesic distances, we report its MSE loss directly.

\begin{table}[!t]

\centering
\caption{Rich Geometric Information}
% We report the average$\pm$std in three random runs.
\label{tab:geo_predict}

\resizebox{\linewidth}{!}{
 \setlength{\tabcolsep}{2.5pt}
\begin{tabular}{c|cccc}
\toprule
Method&Relative Coordinates&Normal Vectors&Geodesic Distances\\
\midrule
PointNet++&58\%&0.26&0.051\\
PointMetaBase&63\%&0.24&0.038\\
\textbf{X-3D}&\textbf{74}\%&\textbf{0.16}&\textbf{0.019}\\
\bottomrule
\end{tabular}
}
% \caption{\textbf{Ablation Study of PointMLP(ours) on different training strategies.}
\end{table}

\begin{figure}[!t]
 \begin{subfigure}[t]{0.15\textwidth}
           \centering
           \includegraphics[width=\textwidth]{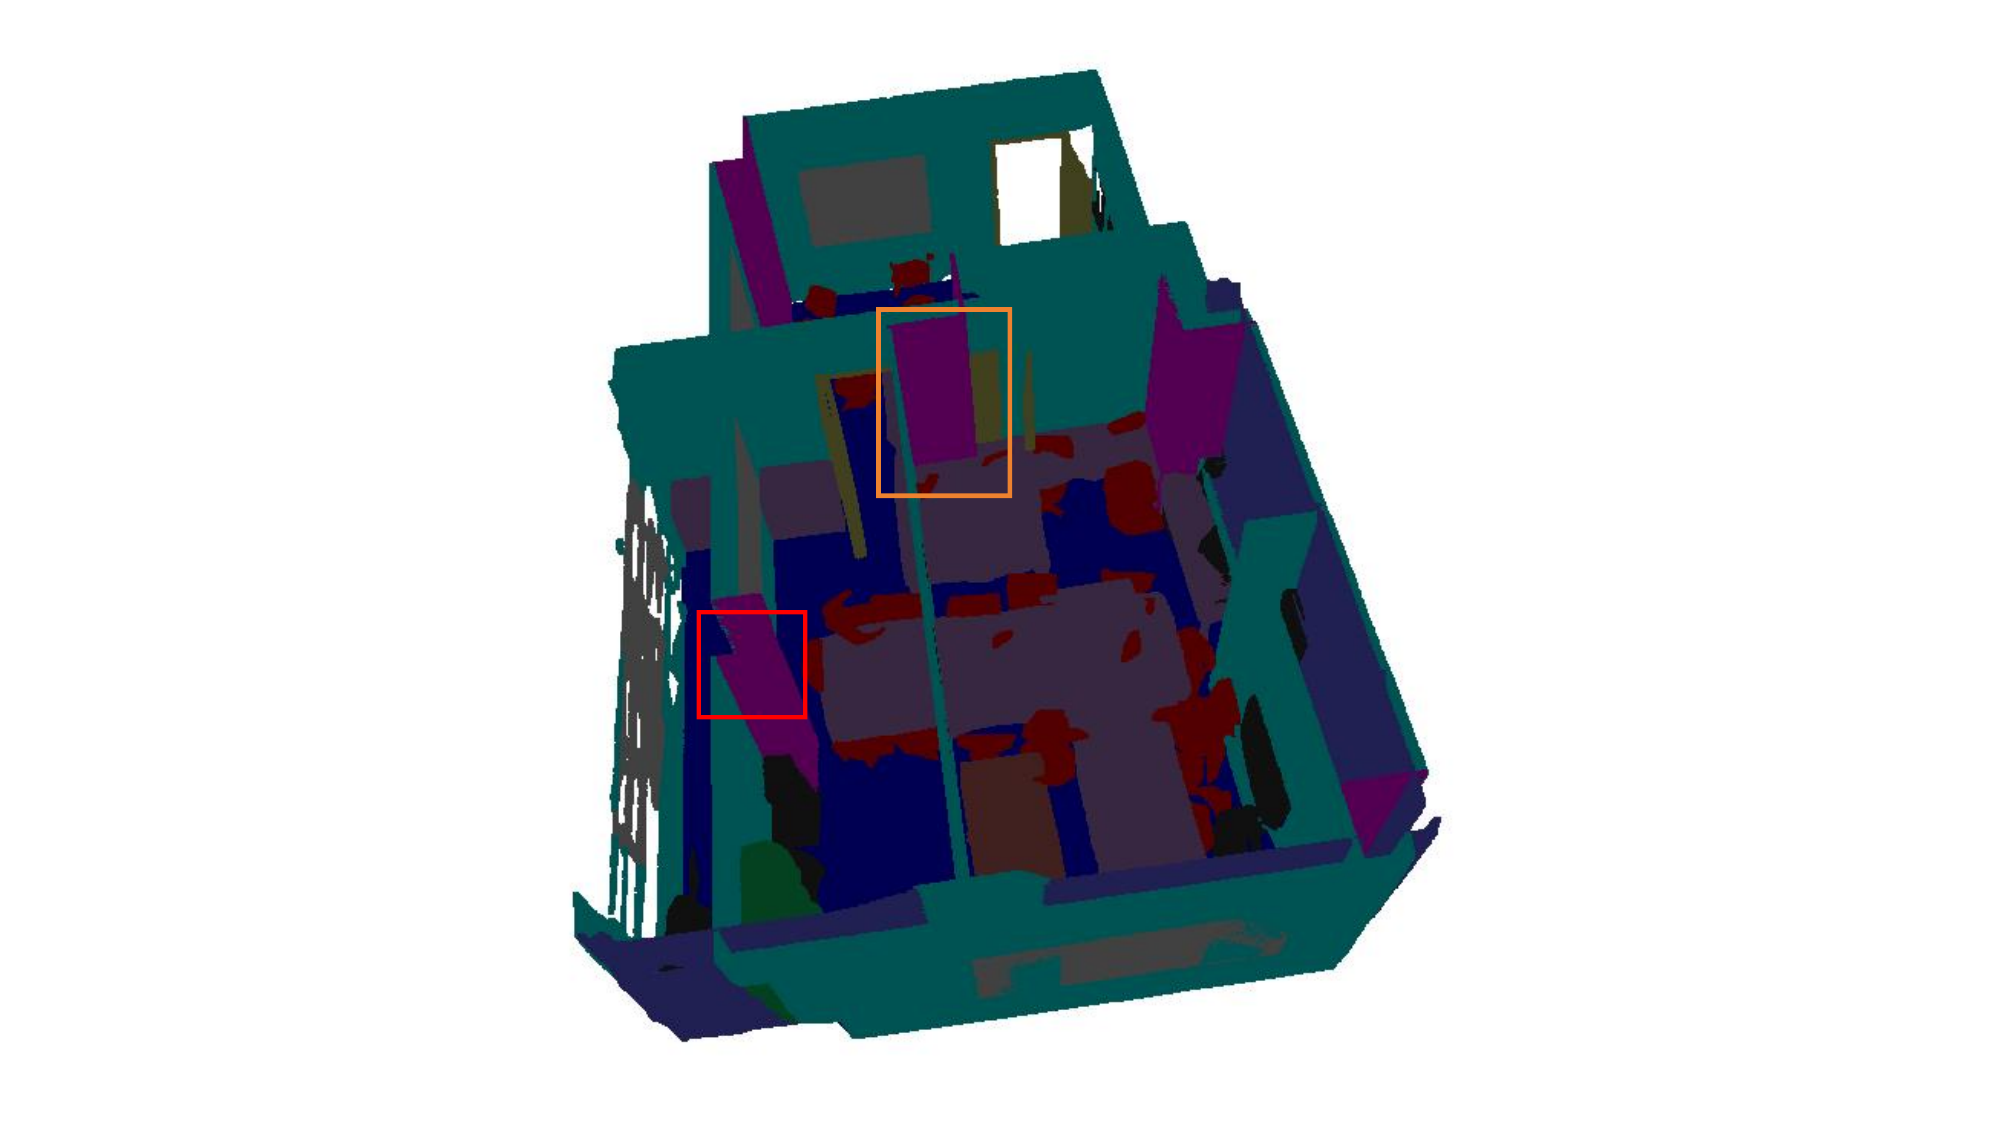}
            \caption{Ground Truth}
           
\end{subfigure}
\begin{subfigure}[t]{0.15\textwidth}
           \centering
           \includegraphics[width=\textwidth]{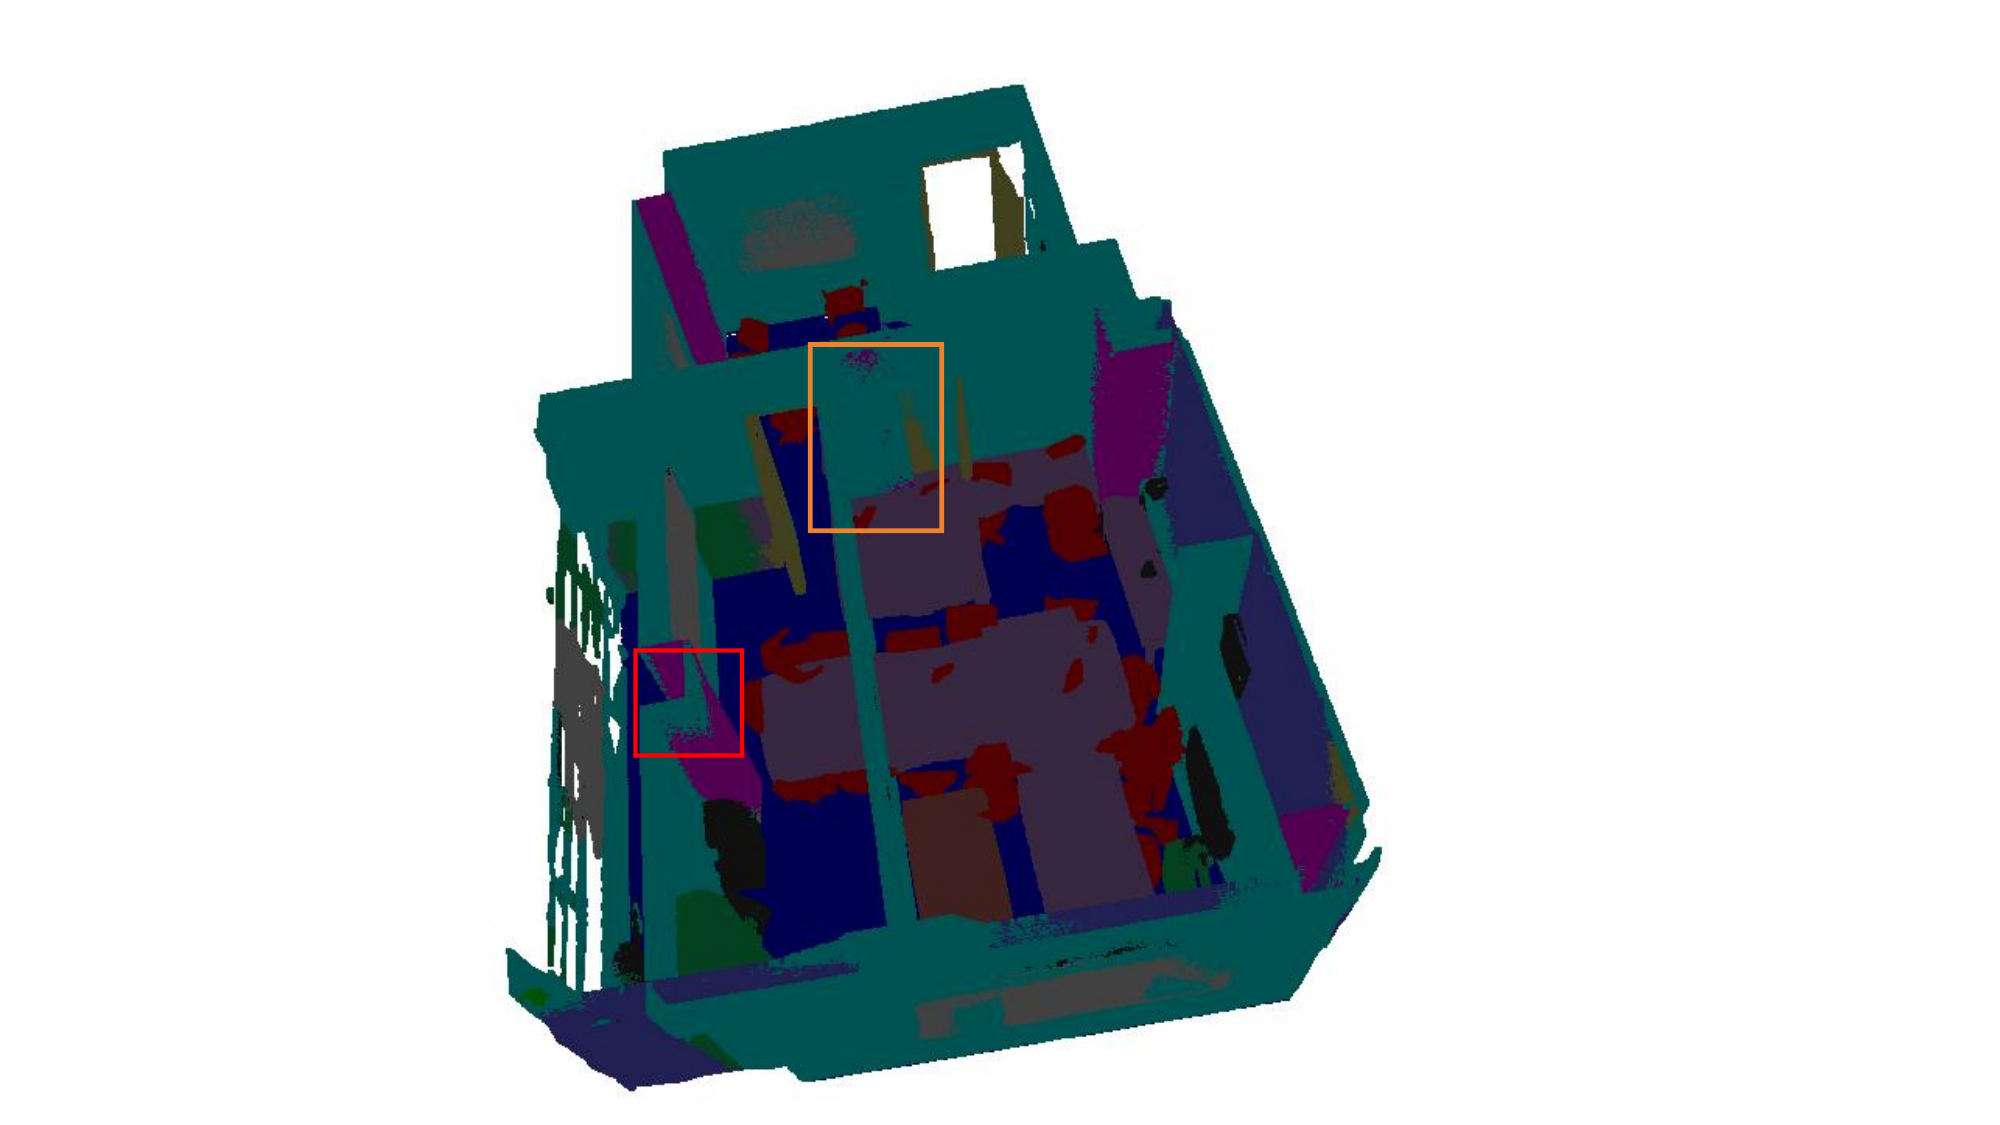}
            \caption{PointMetaBase-L}
            
\end{subfigure}
\begin{subfigure}[t]{0.15\textwidth}
           \centering
           \includegraphics[width=\textwidth]{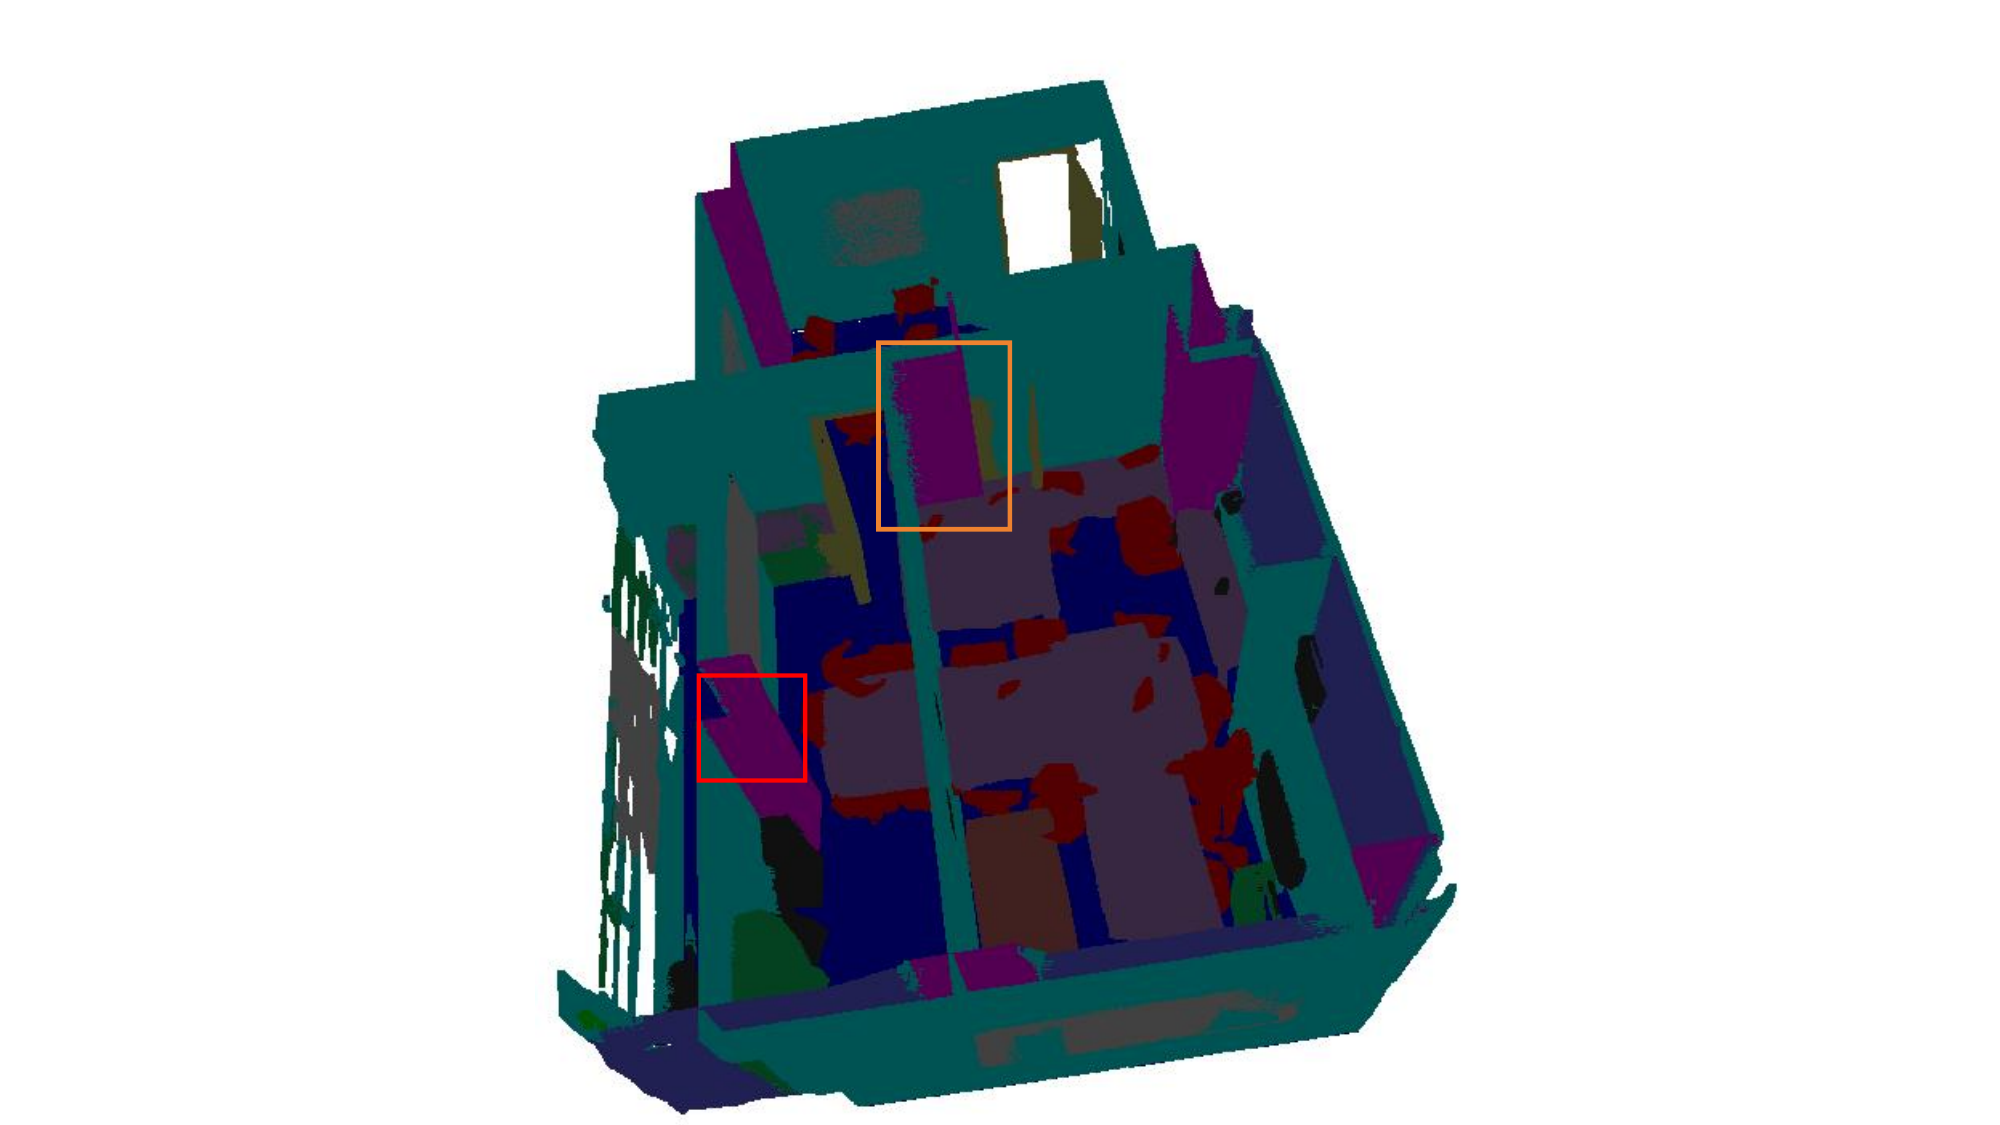}
            \caption{+X-3D}
            
\end{subfigure}
\begin{subfigure}[t]{0.15\textwidth}
        \centering
        \includegraphics[width=\textwidth]{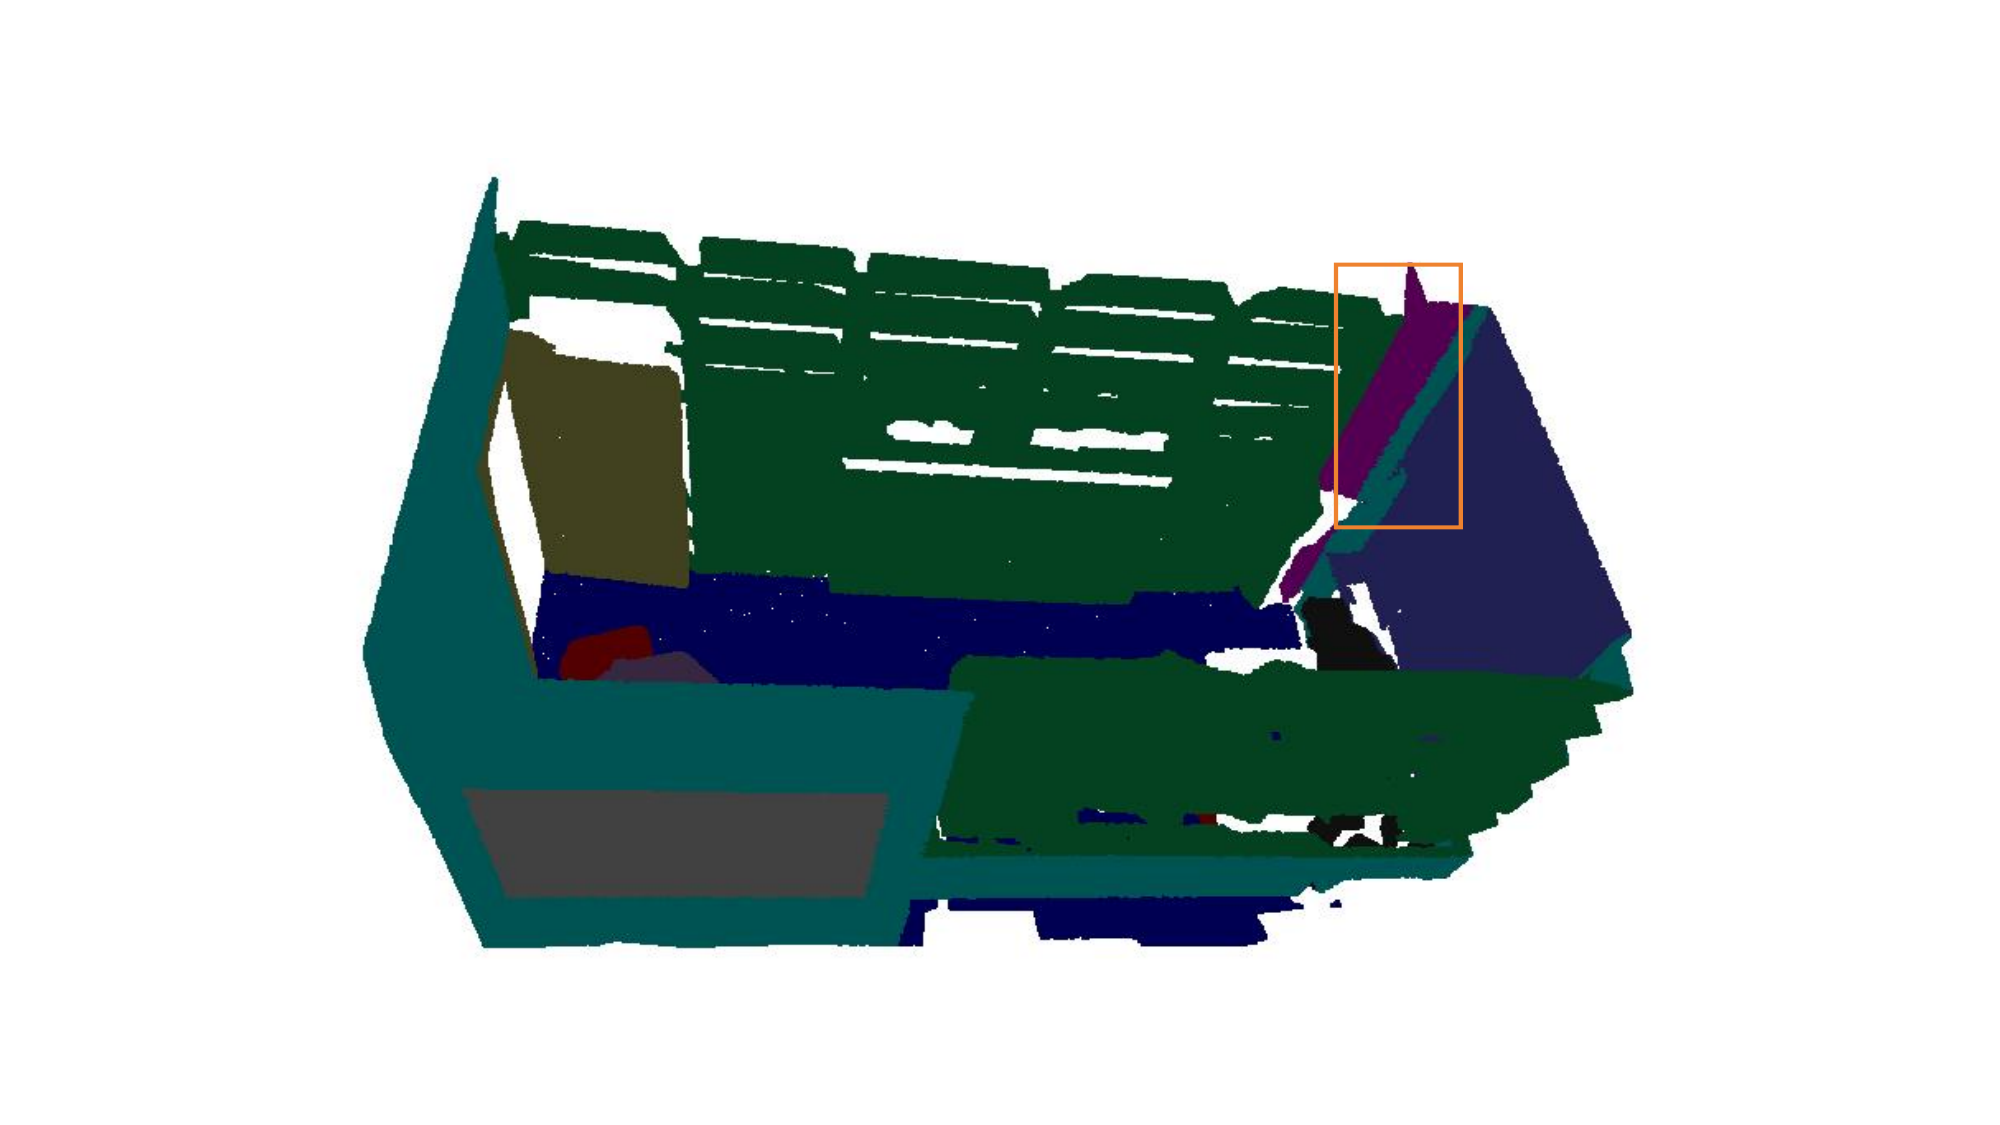}

       \caption{Ground Truth}
        
\end{subfigure}
\begin{subfigure}[t]{0.15\textwidth}
           \centering
           \includegraphics[width=\textwidth]{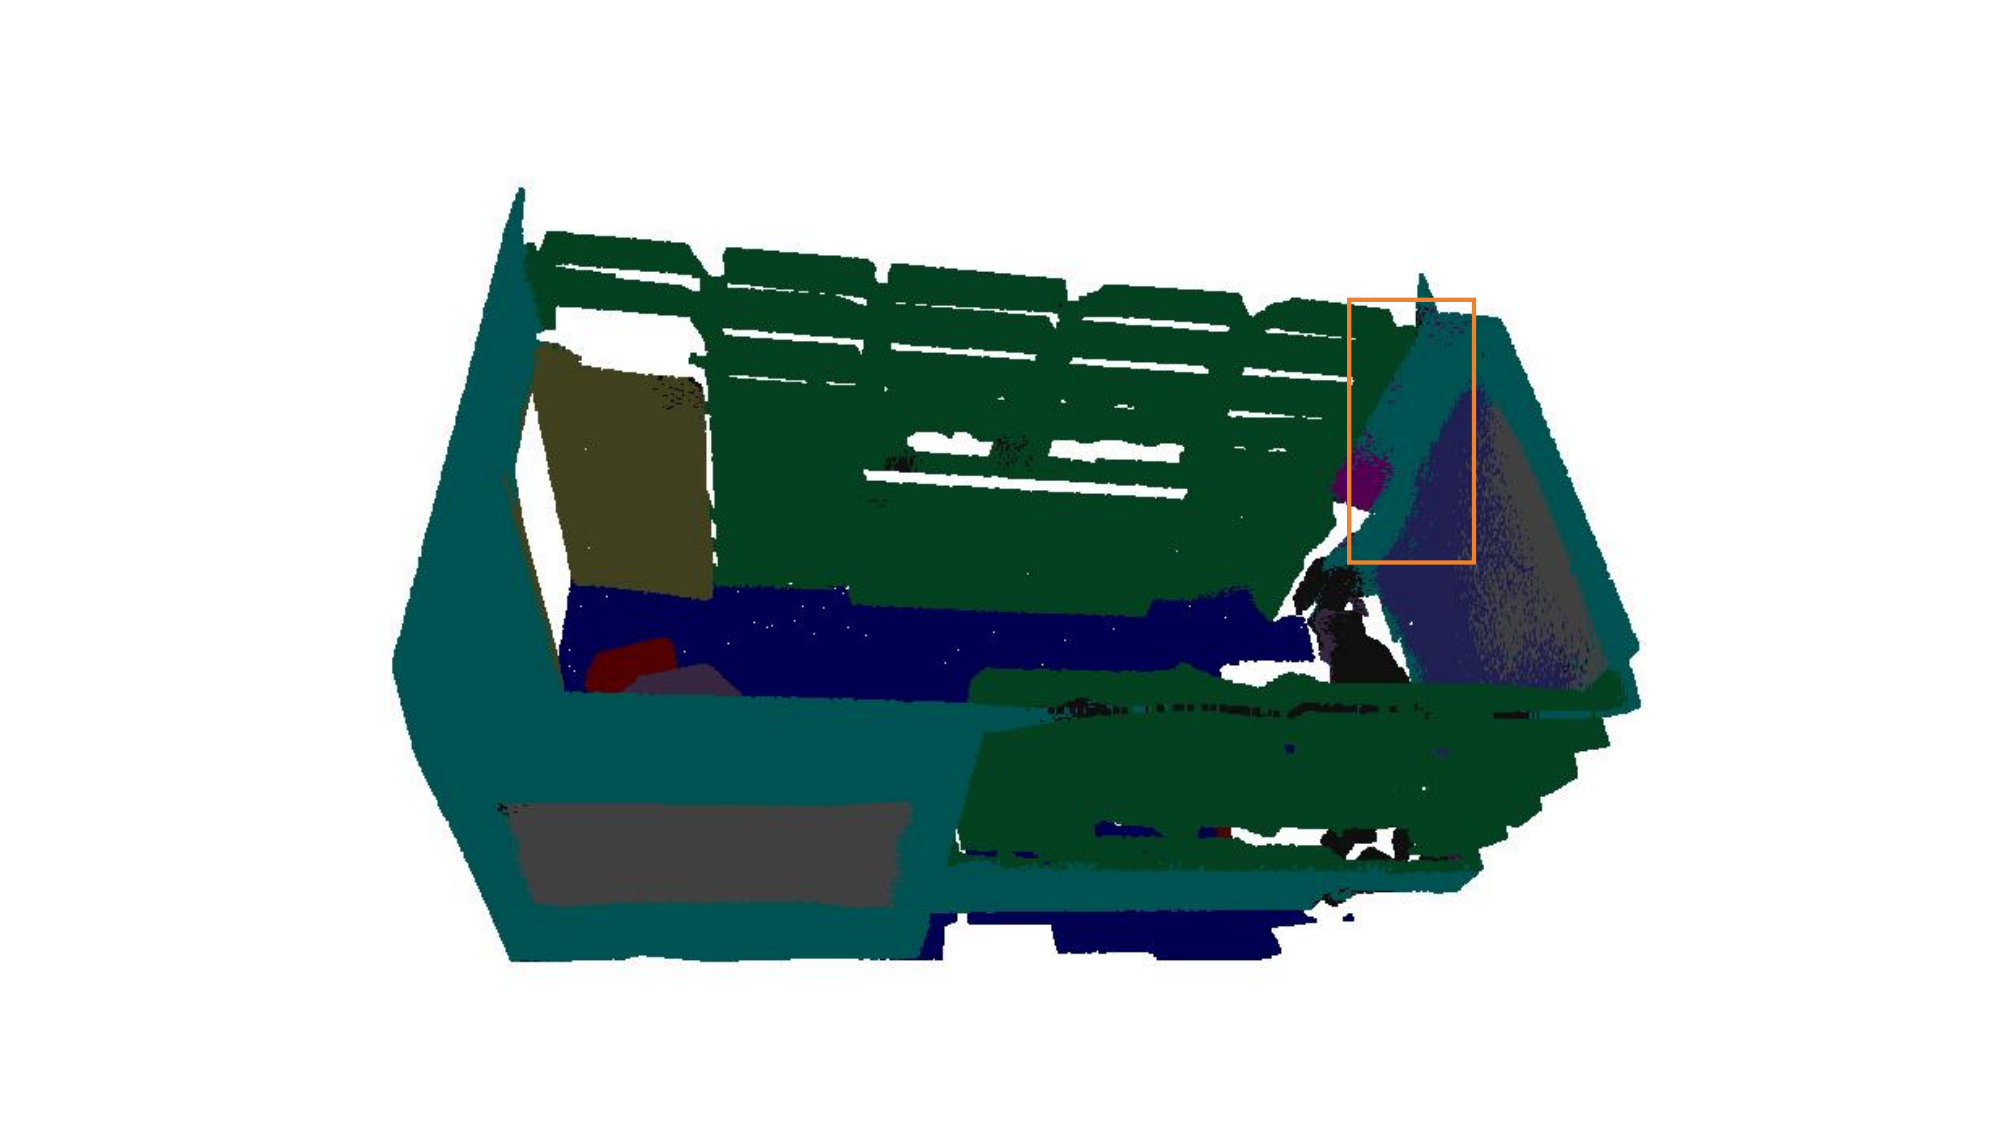}
            \caption{PointMetaBase-L}
            
\end{subfigure}
\begin{subfigure}[t]{0.15\textwidth}
           \centering
           \includegraphics[width=\textwidth]{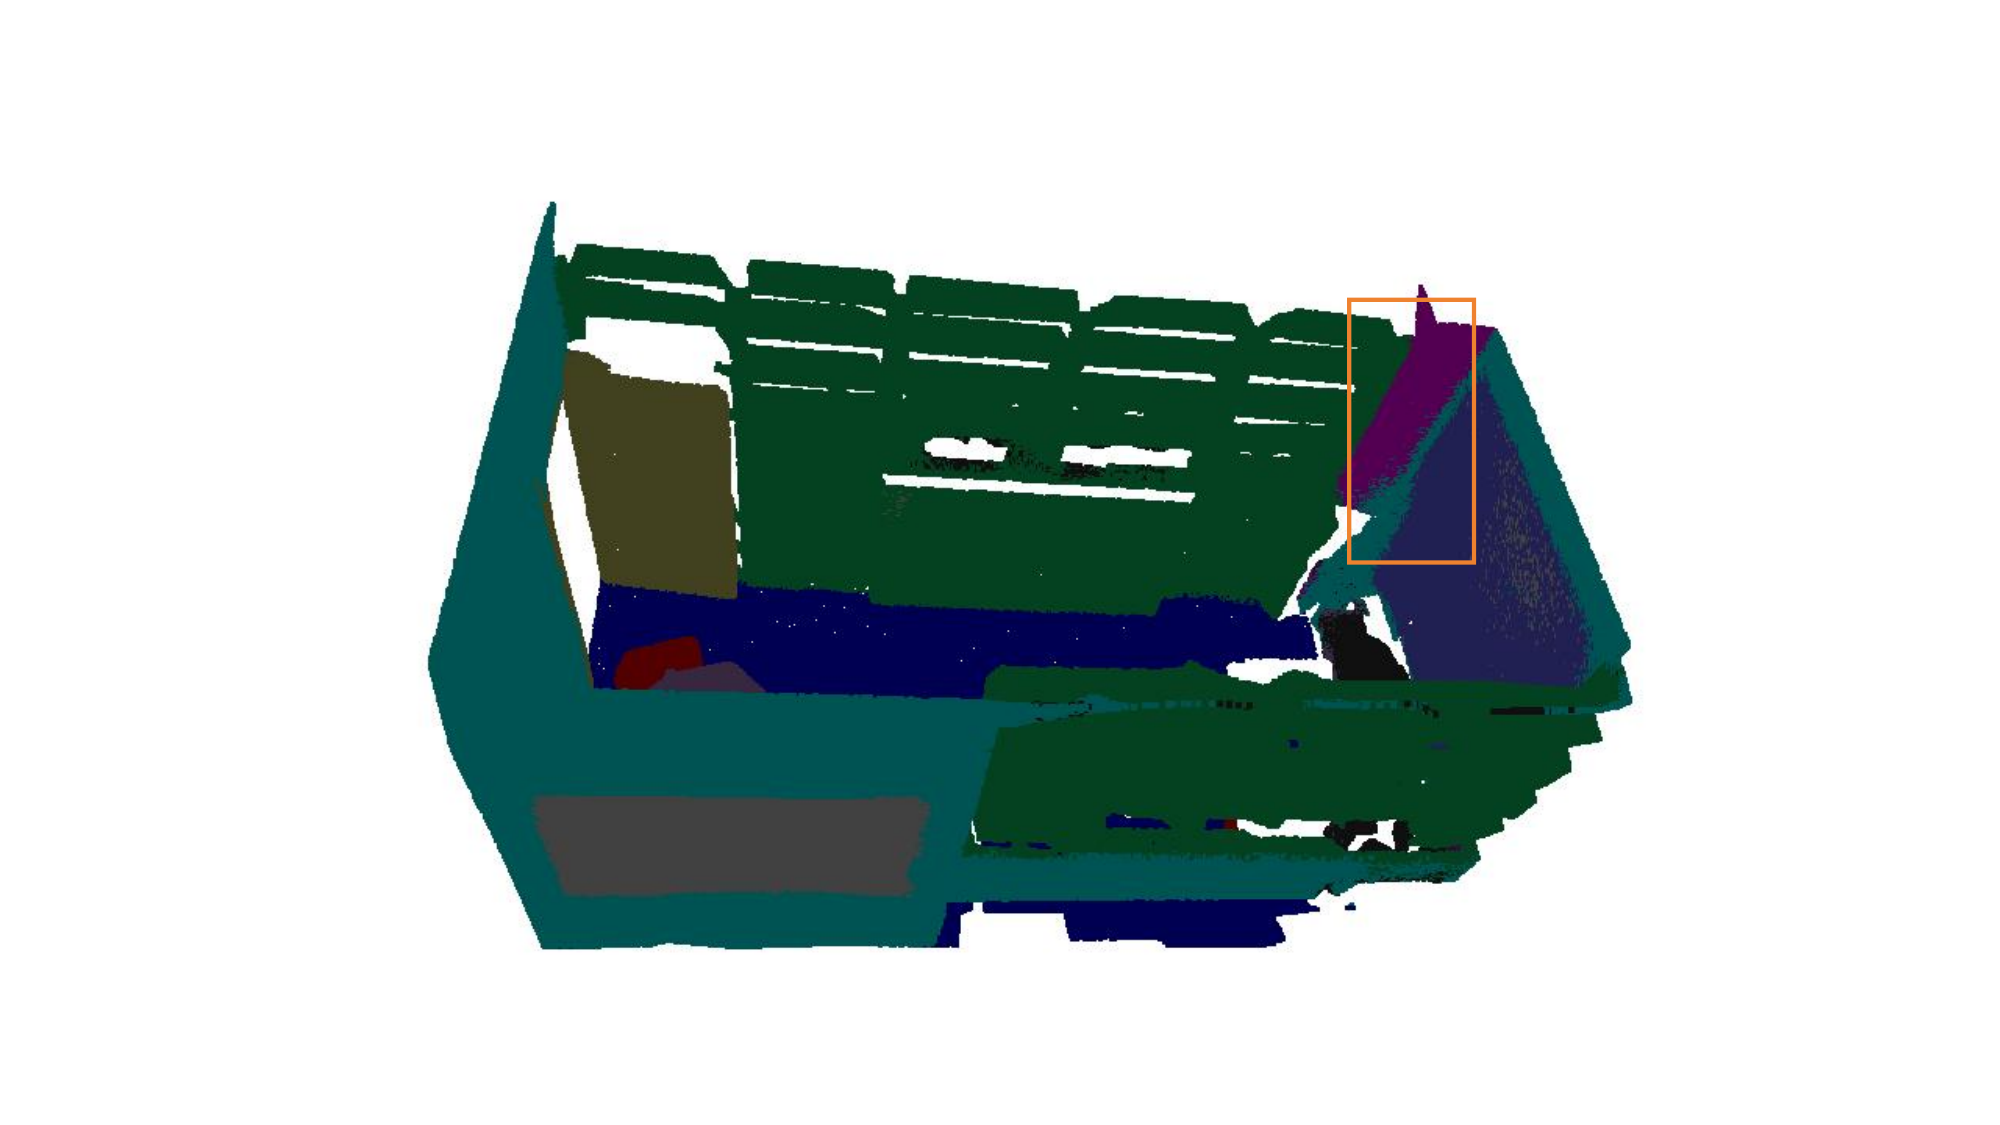}
             \caption{+X-3D}
           
\end{subfigure}
\caption{We visualize the segmentation results of PointMetaBase-L as well as X-3D on S3DIS Area5 and annotate the different places
}\label{fig:vis_result}
\vspace{-1.1em}
\end{figure}

\textbf{Explicit local structure provides strong robustness.} In Table~\ref{tab:rotation}, we report that X-3D is more robust against simple local transformations (rotation, scale). Inspired by ~\cite{ren2022benchmarking}, more powerful data augmentation methods such as cutmix can better study the robustness of point cloud models. Therefore, in this part we use a stronger data augmentation technique, through PointCutmix~\cite{pointcutmix}, to combine different objects by cutmix opearator to achieve the purpose of distorting and occluding the local structure. In Table~\ref{tab:rob_cutmix}, we evaluate PointMetaBase and X-3D on ShapeNetPart using PointCutMix and report the mIoU under different cutmix ratio$\lambda$. Furthermore, we test two cases. The first one uses objects of the same category for cutmix to simulate the local distortion of objects, and the second one uses objects of different categories for cutmix to simulate the occlusion stacking among different objects. Experimental results demonstrate the robustness of X-3D in the face of various difficult situations in real scenes 

\begin{table}[!h]

\centering
\caption{Robustness}
% We report the average$\pm$std in three random runs.
\label{tab:rob_cutmix}

\resizebox{\linewidth}{!}{
 \setlength{\tabcolsep}{2.5pt}
\begin{tabular}{c|ccccc}
\toprule
Method&$\lambda$=0&$\lambda$=0.1&$\lambda$=0.2&$\lambda$=0.3&$\lambda$=0.4\\
\midrule
\multicolumn{6}{c}{Same Category CutMix}\\
\midrule
PointMetaBase&~~~~86.7&~~~~86.5&~~~~84.4&~~~~82.7&~~~~81.2\\
\textbf{X-3D}&~~~~86.9&~~~~86.9&~~~~86.7&~~~~86.0&~~~~85.3\\
\midrule
\multicolumn{6}{c}{Different Category CutMix}\\
\midrule
PointMetaBase&~~~~86.7&~~~~70.3&~~~~51.6&~~~~36.6&~~~~27.7\\
\textbf{X-3D}&~~~~86.9&~~~~80.1&~~~~71.8&~~~~59.2&~~~~46.1\\
\bottomrule

\end{tabular}
}
% \caption{\textbf{Ablation Study of PointMLP(ours) on different training strategies.}
\end{table}

\begin{table}[!h]

\centering
\caption{ We tested the difference between the implicit local structure of the feature Spaces at different layers and the explicit space of the input 3D space on PointMetaBase.}
% We report the average$\pm$std in three random runs.
\label{tab:diff_supp}

\resizebox{0.9\linewidth}{!}{
 \setlength{\tabcolsep}{2.5pt}
\begin{tabular}{c|cccc}

&layer1&layer2&layer3&layer4\\
\midrule
GAP&~~~~1.36&~~~~3.23&~~~~5.37&~~~~7.02\\
\bottomrule
\end{tabular}
}
% \caption{\textbf{Ablation Study of PointMLP(ours) on different training strategies.}
\end{table}

\textbf{Explicit structure provides 3D geometric information that is missing from the feature space.} Most of the existing works can be classified as implict high-dimensional structure modeling, which leads to more and more serious loss of explicit 3D geometric information with the increasing depth of the model, which is shown in Table~\ref{tab:diff_supp}. Therefore,  by explicitly introducing local structure, X-3D supplements the deep feature space with 3D geometric information, which effectively improves the performance

\section{Visualization}
As shown in Fig~\ref{fig:vis_result}, we visualize the segmentation results on S3DIS and can see that X-3D segmentation prediction is generally more complete and accurate due to the introduction of explicit local structure information.

% \section{Rationale}
% \label{sec:rationale}
% % 
% Having the supplementary compiled together with the main paper means that:
% % 
% \begin{itemize}
% \item The supplementary can back-reference sections of the main paper, for example, we can refer to \cref{sec:intro};
% \item The main paper can forward reference sub-sections within the supplementary explicitly (e.g. referring to a particular experiment); 
% \item When submitted to arXiv, the supplementary will already included at the end of the paper.
% \end{itemize}
% % 
% To split the supplementary pages from the main paper, you can use \href{https://support.apple.com/en-ca/guide/preview/prvw11793/mac#:~:text=Delete%20a%20page%20from%20a,or%20choose%20Edit%20%3E%20Delete).}{Preview (on macOS)}, \href{https://www.adobe.com/acrobat/how-to/delete-pages-from-pdf.html#:~:text=Choose%20%E2%80%9CTools%E2%80%9D%20%3E%20%E2%80%9COrganize,or%20pages%20from%20the%20file.}{Adobe Acrobat} (on all OSs), as well as \href{https://superuser.com/questions/517986/is-it-possible-to-delete-some-pages-of-a-pdf-document}{command line tools}.
